# Supplementary material for: Electronics and Optics of Graphene Nanoflakes: Edge Functionalization and Structural Distortions
Source: arXiv:1208.4228 source file (2012-08-21)
Supplement: Supplementary file 1 [file supp-info.pdf]

# SUPPORTING INFORMATION

# Electronics and Optics of Graphene Nanoflakes: Edge Functionalization and Structural Distortions

Caterina Cocchi,[*,†,‡] Deborah Prezzi,[*,†] Alice Ruini,[†,‡] Marilia J. Caldas,[¶] and Elisa Molinari[†,‡]

*Centro S3, CNR-Istituto Nanoscienze, I-41125 Modena, Italy, Dipartimento di Fisica, Università di Modena e Reggio Emilia, I-41125 Modena, Italy, and Instituto de Física, Universidade de São Paulo, 05508-900 São Paulo, SP, Brazil*

E-mail: caterina.cocchi@unimore.it; deborah.prezzi@unimore.it

[*]To whom correspondence should be addressed
[†]Centro S3, CNR-Istituto Nanoscienze, I-41125 Modena, Italy
[‡]Dipartimento di Fisica, Università di Modena e Reggio Emilia, I-41125 Modena, Italy
[¶]Instituto de Física, Universidade de São Paulo, 05508-900 São Paulo, SP, Brazil

The Supporting Information is organized in three sections. In the first one we report the structural details (bond lengths and distortion angles) of the optimized *N*=7, *N*=8 and *N*=9 graphene nanoflakes (GNFs), to complete the data reported in the main text. The second section supports the analysis on the electronic properties, including a table with the dipole moment components of *N*=8 and *N*=9 GNFs (functionalized according to both A-A and A-B schemes) and the isosurfaces of the frontier orbitals for the considered systems. The last part is dedicated to optical properties. The analysis on the effects related to different functionalization schemes and structural distortions are extended here also to $COCH_3$ and F terminations, as representatives of the classes of C-bonded and halogen substituents. We also include the tables with the composition of the main excitations for *N*=8 and *N*=9 GNFs, and the analysis of the optical features of full halogen-terminated GNFs (only *N*=7).

## Structural Properties

We report in Table S1 and Table S2 the bond lengths – C-C and C-X bonds, respectively, with X=F, Cl, Br, N, O, C, depending on the functional group – at the edge of functionalized graphene nanoflakes (GNFs).

**Table S1: C-C bond length (in Å) at the edge of each considered functionalized GNF, optimized with AM1 model. The case of H termination is also reported as a reference.**

| C-C bond length | | | | | | | | | | |
|---|---|---|---|---|---|---|---|---|---|---|
| **H** | **Halogens** | | | **Direct bond** | | | **C-bond** | | | |
| | F | Cl | Br | $NH_2$ | $OCH_3$ | $OCF{=}CF_2$ | $COCH_3$ | $CH{=}CH_2$ | $CH{=}CF_2$ |
| 1.40 | 1.38 | 1.38 | 1.38 | 1.40 | 1.38 | 1.37 | 1.38 | 1.38 | 1.38 |

**Table S2: Bond lengths (in Å) between edge C atoms and functional groups for each considered functionalization.**

| **Halogen** | | | **Direct bond** | | | **C bond** | | |
|---|---|---|---|---|---|---|---|---|
| F | Cl | Br | N | O | | C | | |
| | | | | $OCH_3$ | $OCF{=}CF_2$ | $COCH_3$ | $CH{=}CH_2$ | $CH{=}CF_2$ |
| 1.39 | 1.70 | 1.88 | 1.40 | 1.38 | 1.40 | 1.49 | 1.46 | 1.45 |

In Table S3 we report the values of the distortion angle $\alpha$ for *N*=8 and *N*=9 functionalized

GNFs with selected substituents (F, $NH_2$ and $COCH_3$) for both A-A and A-B schemes. As introduced in the main text, $\alpha$ is defined as the maximum deviation from planarity of edge C atoms in functionalized GNFs. By inspecting Table S3 we notice that in general, as discussed for $N$=7 GNFs in the main text, larger distortions are noticed also for $N$=8 and $N$=9 GNFs in the schemes corresponding to lower symmetry models (A-B and A-A, respectively).

**Table S3: Distortion angle $\alpha$, expressed in degrees, of optimized GNFs of width parameter $N$=8 and $N$=9, functionalized with selected groups (F, $NH_2$ and COCH) according to both schemes. For F termination, the case of full functionalization is also addressed. The angle $\alpha$ represents the maximum deviation of edge C atoms from the planar configuration of the reference H-terminated flake.**

| | $N$=8 | | | $N$=9 | | |
|---|---|---|---|---|---|---|
| | F | $NH_2$ | $COCH_3$ | F | $NH_2$ | $COCH_3$ |
| A-A | 7.2 | 17.8 | 12.5 | 9.4 | 24.7 | 9.3 |
| A-B | 36.8 | 38.4 | 22.2 | 4.9 | 10.1 | 13.5 |
| full | 9.0 | - | - | 21.4 | - | - |

# Electronic Properties

In Table S4 we report the components of the dipole moments of functionalized GNFs of width parameters $N$=8 and $N$=9 for both A-A and A-B scheme. As discussed in the main text, we notice that in general a non negligible dipole component along the longitudinal axis ($\mu_x$) appears in the scheme corresponding to the lower nominal symmetry (A-B for $N$=8 and A-A for $N$=9). The sign of $\mu_x$ is determined by the electronegativity of the substituents. The results are basically in agreement with those discussed in the main text for $N$=7.

**Table S4: Dipole components of funcitonalized GNFs of width parameter *N*=8 and *N*=9: one substituent per class is considered for both A-A and A-B schemes.**

| | Group | Scheme | $\mu_x$ [D] | $\mu_y$ [D] | $\mu_z$ [D] |
|---|---|---|---|---|---|
| *N*=8 | F | A-A | 0.005 | -0.001 | -0.819 |
| | | A-B | 1.212 | 0.299 | 0.675 |
| | $NH_2$ | A-A | -0.260 | -0.081 | 0.116 |
| | | A-B | -16.317 | -0.168 | -0.691 |
| | $COCH_3$ | A-A | -1.964 | 1.536 | -0.414 |
| | | A-B | 8.190 | 0.240 | -0.191 |
| *N*=9 | F | A-A | 7.409 | 0.002 | 0.076 |
| | | A-B | 0.000 | 0.008 | 0.187 |
| | $NH_2$ | A-A | -2.815 | 0.260 | -2.321 |
| | | A-B | -1.191 | 0.970 | 1.594 |
| | $COCH_3$ | A-A | 9.806 | 0.034 | 0.200 |
| | | A-B | -2.128 | -1.914 | 0.105 |

We present the isosurfaces of the frontier orbitals of *N*=7 (Figure S1), *N*=8 and *N*=9 GNFs (Figure S2) for the functionalized systems analyzed in the main text. For consistency, A-B (A-A) scheme is addressed for flakes with odd (even) *N*.

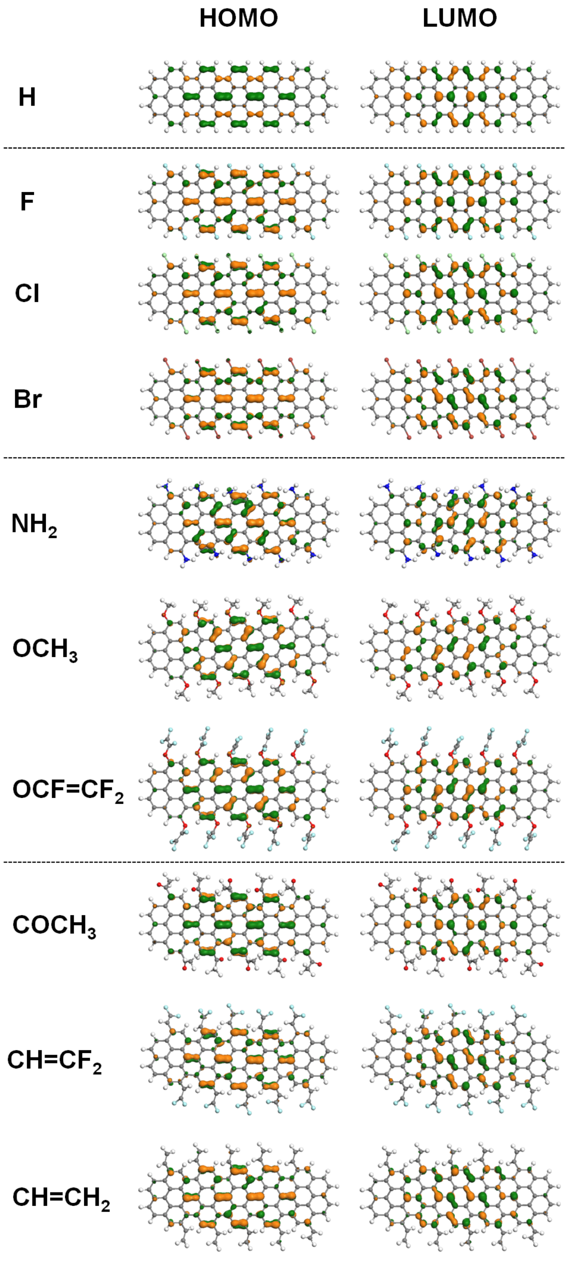


Figure S1: Isosurfaces of the frontier orbitals of functionalized GNFs ($N$=7) according to the A-B scheme. The orbitals of the reference H-terminated system are included for comparison.

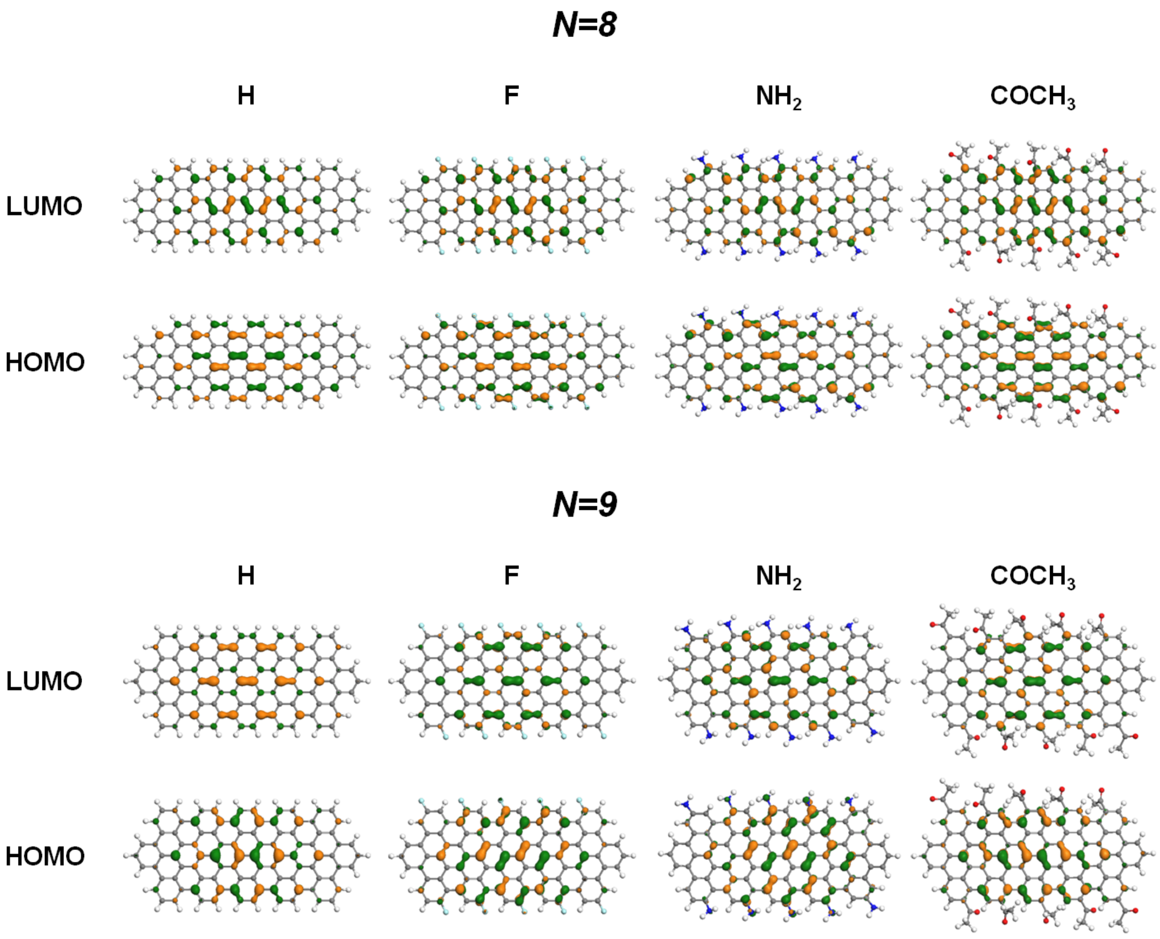


Figure S2: Isosurfaces of frontier molecular orbitals of functionalized GNFs of width parameters *N*=8 (*top*) and *N*=9 (*bottom*). The frontier orbitals of the reference H-terminated system are included for comparison. The A-A (A-B) scheme is addressed for *N*=8 (*N*=9).

# Optical Properties

To supplement the analysis on functionalization-induced distortion effects on the optical properties of GNFs, we include in Figure S3 the optical spectra of $N$=7 GNFs, functionalized by means of $COCH_3$ groups [panels (a-b)] and F atoms [panels (c-d)]. In addition to the spectra of functionalized GNFs (solid lines), we include also those of the H-terminated distorted model structures, obtained by removing edge substituents from the final structure and then H-passivating the remaining dangling bonds (dashed lines); the spectrum of the reference H-terminated GNF is represented in the background of each panel (grey shaded area). Unlike $NH_2$-functionalization (see also Figure 4 in the main text), here the spectra corresponding to the two schemes are basically identical for both substituent species, as suggested also from the similar geometry obtained in the two cases (see main text, Figure 2b for $COCH_3$, and the values of the distortion angle $\alpha$ in Table 1). Compared to the reference H-GNF, we notice for all the spectra a red shift of P1 (about 150 meV) and of P2 (about 100 meV). Most part of these red shift effects (about 80%) is to be ascribed to structural distortions, as shown by the dashed spectra of the H-terminated distorted model flakes.

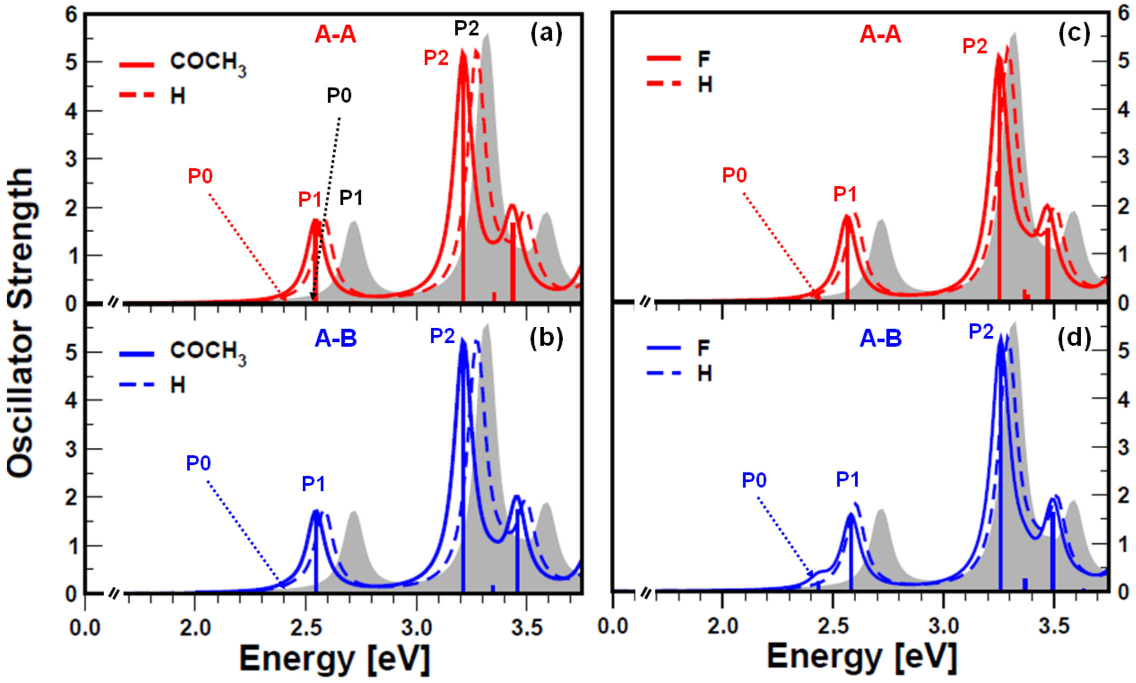


Figure S3: Optical spectra of GNFs of width parameter N=7, functionalized with $COCH_3$ (a-b) and F (c-d), according to the A-A and A-B schemes. In addition to the spectrum of the planar H-terminated flake taken as reference [grey shaded area, with the main excitations highlighted in (a)], we show the spectrum of model GNFs obtained by removing the edge substituents from the final structures and H-passivating the dangling bonds (dashed lines), in order to perform a rigorous analysis of distortions effects.

In Table S5 and Table S6 we report the composition of the main excitations of functionalized GNFs of width parameters $N$=8 and $N$=9, respectively. The corresponding spectra are shown in the main text (Figure 6).

**Table S5: Energy, oscillator strength (OS) and composition of the two lowest energy excitations of functionalized GNFs of width parameter $N$=8 (A-A scheme, see spectra in Figure 6a of the main text). In the last column only the molecular orbital transitions with relative weights larger than 0.1 are reported.**

| System | Excitation | Energy [eV] | OS | Transitions (weight) |
|---|---|---|---|---|
| H | P1 | 1.84 | 3.33 | H → L (0.91) |
| | P2 | 3.64 | 3.47 | H-2 → L+2 (0.56) |
| F | P1 | 1.76 | 3.22 | H → L (0.91) |
| | P2 | 3.56 | 3.62 | H-2 → L+2 (0.62) |
| $NH_2$ | P1 | 1.69 | 3.04 | H → L (0.91) |
| | P2 | 3.04 | 1.64 | H-2 → L (0.46)<br>H → L+2 (0.18)<br>H → L+4 (0.15) |
| $COCH_3$ | P1 | 1.73 | 3.22 | H → L (0.91) |
| | P2 | 3.14 | 1.08 | H-2 → L+1 (0.23)<br>H-2 → L (0.10)<br>H → L+4 (0.26)<br>H → L+6 (0.13) |

**Table S6: Energy, oscillator strength (OS) and composition of the two lowest energy excitations of functionalized GNFs of width parameter $N$=9 (A-B scheme, see spectra in Figure 6b of the main text). In the last column only the molecular orbital transitions with relative weights larger than 0.1 are reported.**

| System | Excitation | Energy [eV] | OS | Transitions (weight) |
|---|---|---|---|---|
| H | P0 | 2.40 | 0.00 | H-1 $\rightarrow$ L (0.37)<br>H $\rightarrow$ L+1 (0.41) |
| | P1 | 2.47 | 1.71 | H $\rightarrow$ L (0.85) |
| | P2 | 3.24 | 4.47 | H-2 $\rightarrow$ L+2 (0.12)<br>H-1 $\rightarrow$ L+1 (0.73) |
| F | P0 | 2.34 | 0.06 | H-1 $\rightarrow$ L (0.36)<br>H $\rightarrow$ L+1 (0.39) |
| | P1 | 2.48 | 1.31 | H $\rightarrow$ L (0.78) |
| | P2 | 3.12 | 4.80 | H-1 $\rightarrow$ L+1 (0.69) |
| $NH_2$ | P1 | 2.17 | 0.76 | H $\rightarrow$ L (0.55)<br>H $\rightarrow$ L+1 (0.12) |
| | P0 | 2.44 | 0.50 | H-1 $\rightarrow$ L (0.27)<br>H $\rightarrow$ L (0.24)<br>H $\rightarrow$ L+1 (0.33) |
| | P2 | 3.03 | 4.64 | H-1 $\rightarrow$ L+1 (0.57) |
| $COCH_3$ | P0 | 2.33 | 0.01 | H-1 $\rightarrow$ L (0.37)<br>H $\rightarrow$ L+1 (0.41) |
| | P1 | 2.48 | 1.21 | H $\rightarrow$ L (0.80) |
| | P2 | 3.08 | 4.55 | H-1 $\rightarrow$ L+1 (0.64) |

We finally present the results on the optical properties of fully functionalized $N$=7 GNFs with halogen terminations. In Figure S4(a) we show the computed spectra, where the main excitations are indicated for the reference H-GNF (grey shaded area). In case of full functionalization the model symmetry of the H-terminated flake is preserved and hence the character of the frontier orbitals [see Figure S4(b)] as well as the composition of the main excitations in terms of molecular orbital transitions and their intensity are not significantly affected (see Table S7). A red shift of the spectra (about 350 meV for P1 and about 250 meV for P2) is noticed, compared to the reference H-GNF.

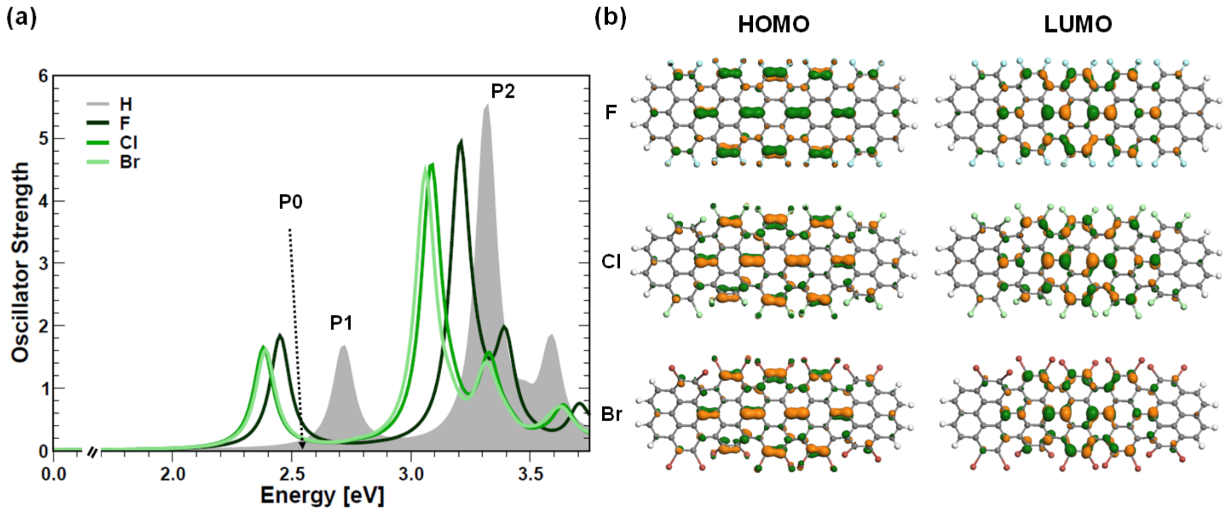


Figure S4: (a) Optical spectra of $N$=7 graphene nanoflakes fully functionalized with halogen atoms. For comparison, the spectrum of the reference H-terminated flake is included (grey shaded area with the labels of the main excitations). (b) Frontier orbitals of the corresponding structures.

**Table S7: Energy, oscillator strength (OS) and composition of the main excitations (P0, P1 and P2) of fully functionalized *N*=7 GNFs with halogen terminations (F, Cl, Br – see Figure S5). In the last column only the molecular orbital transitions with relative weights larger than 0.1 are reported.**

| System | Excitation | Energy [eV] | OS | Transitions (weight) |
|---|---|---|---|---|
| H | P0 | 2.54 | 0.0005 | H-1 → L (0.37)<br>H → L+1 (0.39) |
| | P1 | 2.72 | 1.62 | H → L (0.79) |
| | P2 | 3.32 | 5.43 | H-3 → L+3 (0.12)<br>H-1 → L+1 (0.76) |
| F | P0 | 2.36 | 0.02 | H-1 → L (0.30)<br>H → L+1 (0.45) |
| | P1 | 2.45 | 1.81 | H → L (0.82) |
| | P2 | 3.21 | 4.70 | H-3 → L+3 (0.11)<br>H-2 → L+1 (0.73) |
| Cl | P0 | 2.27 | 0.01 | H-1 → L (0.28)<br>H → L+1 (0.42) |
| | P1 | 2.38 | 1.62 | H → L (0.81) |
| | P2 | 3.08 | 4.42 | H-3 → L+2 (0.10)<br>H-1 → L+1 (0.67) |
| Br | P0 | 2.27 | 0.01 | H-1 → L (0.29)<br>H → L+1 (0.42) |
| | P1 | 2.39 | 1.59 | H → L (0.81) |
| | P2 | 3.06 | 4.33 | H-3 → L+2 (0.10)<br>H-1 → L+1 (0.69) |
